# Supplementary material for: Glimpse Clouds: Human Activity Recognition from Unstructured Feature Points
Source: arXiv:1802.07898 source file (2018-08-21)
Supplement: Supplementary file 1 [file sec_7_supplementary.tex]

\section{Supplementary materials}
\label{sec:supplementary}
